# Supplementary material for: Dual Contrastive Learning for Unsupervised Image-to-Image Translation
Source: arXiv:2104.07689 source file (2021-04-15)
Supplement: Supplementary file 1 [file supp1.tex]

\begin{figure*}[htb]
  \begin{minipage}[t]{0.245\linewidth} 
    \centering 
    \text{Input}
  \end{minipage} 
    \begin{minipage}[t]{0.245\linewidth} 
    \centering 
    \text{DCLGAN}
  \end{minipage} 
    \begin{minipage}[t]{0.245\linewidth} 
    \centering 
      \text{Variant}
  \end{minipage} 
    \begin{minipage}[t]{0.245\linewidth} 
    \centering 
        \text{Label}
  \end{minipage} 
  \\
    \begin{minipage}[t]{0.245\linewidth} 
    \centering 
    \includegraphics[width=1.65in, height=1in]{ 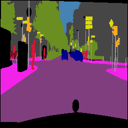}
  \end{minipage} 
    \begin{minipage}[t]{0.245\linewidth} 
    \centering 
    \includegraphics[width=1.65in, height=1in]{ 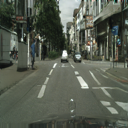}
  \end{minipage} 
      \begin{minipage}[t]{0.245\linewidth} 
    \centering 
    \includegraphics[width=1.65in, height=1in]{ 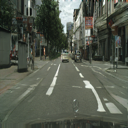}
  \end{minipage} 
    \begin{minipage}[t]{0.245\linewidth} 
    \centering 
    \includegraphics[width=1.65in, height=1in]{ 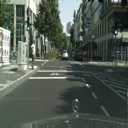}
  \end{minipage} 
  \\
    \begin{minipage}[t]{0.245\linewidth} 
    \centering 
    \includegraphics[width=1.65in, height=1in]{ 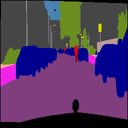}
  \end{minipage} 
    \begin{minipage}[t]{0.245\linewidth} 
    \centering 
    \includegraphics[width=1.65in, height=1in]{ 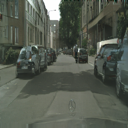}
  \end{minipage} 
      \begin{minipage}[t]{0.245\linewidth} 
    \centering 
    \includegraphics[width=1.65in, height=1in]{ 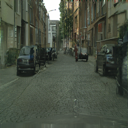}
  \end{minipage} 
    \begin{minipage}[t]{0.245\linewidth} 
    \centering 
    \includegraphics[width=1.65in, height=1in]{ 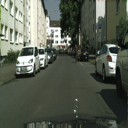}
  \end{minipage} 
  \\
      \begin{minipage}[t]{0.245\linewidth} 
    \centering 
    \includegraphics[width=1.65in, height=1in]{ 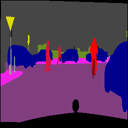}
  \end{minipage} 
    \begin{minipage}[t]{0.245\linewidth} 
    \centering 
    \includegraphics[width=1.65in, height=1in]{ 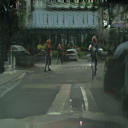}
  \end{minipage} 
      \begin{minipage}[t]{0.245\linewidth} 
    \centering 
    \includegraphics[width=1.65in, height=1in]{ 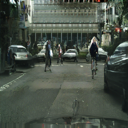}
  \end{minipage} 
    \begin{minipage}[t]{0.245\linewidth} 
    \centering 
    \includegraphics[width=1.65in, height=1in]{ 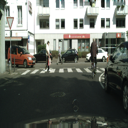}
  \end{minipage} 
  \\
      \begin{minipage}[t]{0.245\linewidth} 
    \centering 
    \includegraphics[width=1.65in, height=1in]{ 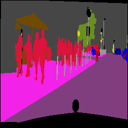}
  \end{minipage} 
    \begin{minipage}[t]{0.245\linewidth} 
    \centering 
    \includegraphics[width=1.65in, height=1in]{ 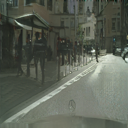}
  \end{minipage} 
      \begin{minipage}[t]{0.245\linewidth} 
    \centering 
    \includegraphics[width=1.65in, height=1in]{ 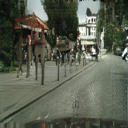}
  \end{minipage} 
    \begin{minipage}[t]{0.245\linewidth} 
    \centering 
    \includegraphics[width=1.65in, height=1in]{ 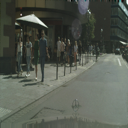}
  \end{minipage} 
 \caption{Comparison between DCLGAN and variant drawing external negatives on task CityScapes.}
  \label{fig:supp1}
\end{figure*}
